# Supplementary material for: Of All StrIPEs: Investigating Structure-informed Positional Encoding for Efficient Music Generation
Source: arXiv:2504.05364 source file (2025-04-07)
Supplement: Supplementary file 1 [file appendix.tex]

\section*{Supplementary Materials}

\noindent\textbf{I. Proof sketch for Proposition 1}, which states that Equation (4) defines attention as a Tensor Product Kernel:
\begin{equation}
    a_{mn}^d = \kappa(q_{md}, k_{nd}) \times \chi_d (p_m, p_n)
\end{equation}\\

\noindent The first step is to notice that the following holds $\forall d \in \{ 1, ..., D \}$:
\begin{equation} \label{eq:sketch_prop1}
    \mathbf{A}_d = \text{diag}(\mathbf{Q}_{:,d}) \mathbf{P}_d \text{diag}(\mathbf{K}_{:,d}) = \mathbf{Q}_{:,d} \mathbf{K}_{:,d}^\top \odot \mathbf{P}_d
\end{equation}
where $\odot$ is the Hadamard product. Then, 
\begin{align}
    a_{mn} &= \left[ \sum_{d=1}^D \text{diag}(\mathbf{Q}_{:,d}) \mathbf{P}_d \text{diag}(\mathbf{K}_{:,d}) \right]_{mn} \\
    &= \left[ \sum_{d=1}^D \mathbf{A}_d \right]_{mn} \\
    &= \sum_{d=1}^D a_{mn}^d \numberthis \label{eq:sketch_prop2}
\end{align}
Then, from Equation \ref{eq:sketch_prop1}, we can write:
\begin{equation} \label{eq:sketch_prop3}
    a_{mn}^d = \kappa(q_{md}, k_{nd}) \times \chi_d (p_m, p_n)
\end{equation}
where $\kappa(q_{md}, k_{nd}) = q_{md} k_{nd}$ and $\chi_d (p_m, p_n) = \left[ \mathbf{P}_d \right]_{mn}$. \qed \\

\noindent\textbf{II. To show that:} F-StrIPE$_1$ has the cross-dimension independence property.\\

\noindent For this, we need to do the following steps:
\begin{enumerate}
    \item Find the complex-valued unpooled feature transform $\mathcal{U}_z(\cdot)$ corresponding to the real-valued unpooled feature transform $\mathcal{U}(\cdot)$, such that $\mathcal{U}(\mathbf{q}_m) \mathcal{U}(\mathbf{k}_n)^\top = \mathfrak{Re} \Big( \mathcal{U}_z(\mathbf{q}_m) \mathcal{U}_z(\mathbf{k}_n)^\top \Big)$ 
    \item Find the complex-valued pooled feature transform $\mathcal{C}_z(\cdot)$ for $\mathcal{U}_z(\cdot)$ and compute the real-valued pooled feature transform $\mathcal{C}(\cdot)$ corresponding to $\mathcal{C}_z(\cdot)$
    \item Show that, since:
    \begin{enumerate}
        \item $\mathcal{U}(\mathbf{q}_m) \mathcal{U}(\mathbf{k}_n)^\top = \mathfrak{Re} \Big( \mathcal{U}_z(\mathbf{q}_m) \mathcal{U}_z(\mathbf{k}_n)^\top \Big)$
        \item $\mathcal{U}_z(\mathbf{q}_m) \mathcal{U}_z(\mathbf{k}_n)^\top = \mathcal{C}_z(\mathbf{q}_m) \mathcal{C}_z(\mathbf{k}_n)^\top$
        \item $\mathcal{C}(\mathbf{q}_m) \mathcal{C}(\mathbf{k}_n)^\top = \mathfrak{Re} \Big( \mathcal{C}_z(\mathbf{q}_m) \mathcal{C}_z(\mathbf{k}_n)^\top \Big)$
    \end{enumerate}
    we have that $\mathcal{U}(\mathbf{q}_m) \mathcal{U}(\mathbf{k}_n)^\top = \mathcal{C}(\mathbf{q}_m) \mathcal{C}(\mathbf{k}_n)^\top$, as desired.
\end{enumerate}

For step 1, we can use equations (17) and (20) from the paper to get the unpooled feature map for F-StrIPE$_1$:
\begin{equation}
    \mathcal{U}(\mathbf{a}_t) : \mathbf{a}_t \mapsto  
    \begin{bmatrix} 
    a_{1} \cos (2 \pi f_1 p_t) \\ 
    a_{1} \sin (2 \pi f_1 p_t) \\ 
    \vdots \\ 
    a_{D} \cos (2 \pi f_D p_t) \\ 
    a_{D} \sin (2 \pi f_D p_t) 
    \end{bmatrix}^\top
\end{equation}
We can calculate the complex-valued unpooled feature map by noting that:
\begin{align}
    \mathcal{U}(\mathbf{q}_m) \mathcal{U}(\mathbf{k}_n)^\top &= \sum_{d=1}^D q_{dm} k_{dn} \cos ( 2 \pi f_{d} ( p_m - p_n ) ) \\
    &= \mathfrak{Re} \big( \sum_{d=1}^D q_{dm} k_{dn} \exp ( 2\pi i f_{d} ( p_m - p_n ) ) \big)
\end{align}
Then, we can derive the complex-valued feature map by expanding the complex-valued sum above as:
% \begin{align}
%     \mathcal{U}_z(\mathbf{a}_t) : \mathbf{a}_t &\mapsto  
%     \begin{bmatrix} 
%     q_{1m} \exp (2 \pi i f_1 p_t) \\ 
%     \vdots \\ 
%     q_{Dm} \exp (2 \pi i f_D p_t) 
%     \end{bmatrix}^\top \\
%     \mathcal{U}_z(\mathbf{k}_n) : \mathbf{k}_n &\mapsto  
%     \begin{bmatrix} 
%     k_{1n} \exp (- 2 \pi i f_1 p_n) \\ 
%     \vdots \\ 
%     k_{Dn} \exp (- 2 \pi i f_D p_n) 
%     \end{bmatrix}^\top
% \end{align}
\begin{equation}
    \mathcal{U}_z(\mathbf{a}_t) : \mathbf{a}_t \mapsto  
    \begin{bmatrix} 
    a_{1t} \exp (2 \pi i f_1 p_t) \\ 
    \vdots \\ 
    a_{Dt} \exp (2 \pi i f_D p_t) 
    \end{bmatrix}^\top
\end{equation}
with the feature transform for queries being $\mathcal{U}_z(\mathbf{q}_m)$ and for keys being $\mathcal{U}^{\dagger}_z(\mathbf{k}_n)$, where $\dagger$ denotes that we take the complex conjugate of $\mathcal{U}_z(\mathbf{k}_n)$ elementwise.
Note that this exactly matches the expected expression for stationary, positive-definite kernels~\cite{rahimi_random_2007}. Clearly, $\mathcal{U}(\mathbf{q}_m) \mathcal{U}(\mathbf{k}_n)^\top = \mathfrak{Re} \Big( \mathcal{U}_z(\mathbf{q}_m) \mathcal{U}_z^\dagger(\mathbf{k}_n)^\top \Big)$.

For step 2, we can find the complex-valued pooled feature transforms for keys and queries by adding up the dimensions of the unpooled complex-valued transform.
% \begin{align}
%     \mathcal{C}_z(\mathbf{q}_m) : \mathbf{q}_m &\mapsto \left[ \sum_{d=1}^D q_{dm} \exp (2 \pi i f_d p_m) \right]^\top \label{eq:complex_feature1} \\
%     \mathcal{C}_z(\mathbf{k}_n) : \mathbf{k}_n &\mapsto \left[ \sum_{d=1}^D k_{dn} \exp (- 2 \pi i f_d p_n) \right]^\top \label{eq:complex_feature2}
% \end{align}
\begin{equation}
    \mathcal{C}_z(\mathbf{a}_t) : \mathbf{a}_t \mapsto \left[ \sum_{d=1}^D a_{dt} \exp (2 \pi i f_d p_t) \right]^\top \label{eq:complex_feature1}
\end{equation}
with the pooled transform for queries being $\mathcal{C}_z (\mathbf{q}_m)$ and for keys being $\mathcal{C}_z^\dagger (\mathbf{k}_n)$.
To write down the real-valued pooled feature transform $\mathcal{C}(\cdot)$, we first write down $ \mathfrak{Re} \big( \mathcal{C}_z(\mathbf{q}_m) \mathcal{C}_z^\dagger(\mathbf{k}_n)^\top \big)$, which is as follows:
\begin{align}
    \mathcal{C}_z(\mathbf{q}_m) : \mathbf{q}_m &\mapsto \left[ \sum_{d=1}^D q_{dm} \big( \cos (2 \pi f_d p_m) + i \sin (2 \pi f_d p_m) \big) \right]^\top \\
    \mathcal{C}_z^\dagger(\mathbf{k}_n) : \mathbf{k}_n &\mapsto \left[ \sum_{d=1}^D k_{dn} \big( \cos (2 \pi f_d p_n) - i \sin (2 \pi f_d p_n) \big) \right]^\top
\end{align}
\begin{equation}
    \begin{split}
    \mathfrak{Re} \big( \mathcal{C}_z(\mathbf{q}_m) \mathcal{C}_z^\dagger(\mathbf{k}_n)^\top \big) = 
    \big( \sum_{d=1}^D &q_{dm} \big( \cos (2 \pi f_d p_m) \big) \\ 
    &\big( \sum_{d^\prime=1}^D k_{d^\prime n} \big( \cos (2 \pi f_{d^\prime} p_n) \big) + \\
    \big( \sum_{d=1}^D &q_{dm} \big( \sin (2 \pi f_d p_m) \big) \\ 
    &\big( \sum_{d^\prime=1}^D k_{d^\prime n} \big( \sin (2 \pi f_{d^\prime} p_n) \big)
    \end{split}
\end{equation}
We can turn this expression into a matrix multiplication form to get:
\begin{equation}
    \mathcal{C}(\mathbf{a}_t) : \mathbf{a}_t \mapsto
    \begin{bmatrix} 
    \sum_{d=1}^D a_d \cos (2 \pi f_d p_t) \\ 
    \sum_{d=1}^D a_d \sin (2 \pi f_d p_t)
    \end{bmatrix}^\top
\end{equation}
Again, by design, we obtain that $\mathcal{C}(\mathbf{q}_m) \mathcal{C}(\mathbf{k}_n)^\top = \mathfrak{Re} \Big( \mathcal{C}_z(\mathbf{q}_m) \mathcal{C}_z^\dagger(\mathbf{k}_n)^\top \Big)$

For step 3, we need to only prove that substeps a, b, and c are true. We already proved 3a and 3c in steps 1 and 2, respectively, above. For 3b, we use a basic fact from harmonic analysis, namely, that complex exponentials with different frequencies are orthogonal, and thus, when we calculate $\mathcal{C}_z(\mathbf{q}_m) \mathcal{C}_z^\dagger(\mathbf{k}_n)^\top$ using equation (\ref{eq:complex_feature1}), the multiplications of the cross-dimension terms terms evaluate to 0. This completes the proof for step 3b. \qed \\

\noindent\textbf{III. Derivation for RoPEPool} corresponding to Equation (23).\\

\noindent Similar to the proof above, we will find $\mathcal{U}(\cdot)$, $\mathcal{C}(\cdot)$, $\mathcal{U}_z(\cdot)$ and $\mathcal{C}_z(\cdot)$ for RoPE. As shown in Fig. \ref{fig:drawing} below, we are interested in the expression $\mathcal{C}(\mathbf{q}_m) \mathcal{C}(\mathbf{k}_n)^\top$, since this will give us the real-valued expression for RoPEPool, as desired in Equation (23).

\begin{figure}[b]
    \centering
    \includegraphics[width=1.75in]{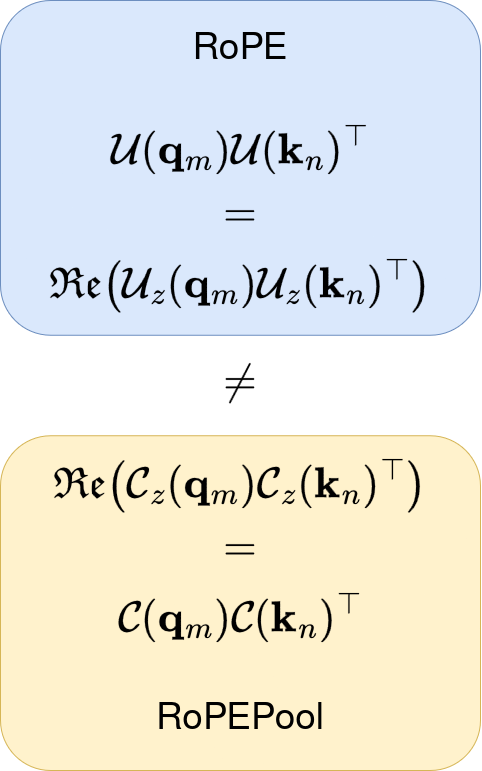}
    \caption{RoPE vs RoPEPool}
    \label{fig:drawing}
\end{figure}

From equations (21) and (22) in the paper, we can find the complex-valued counterpart $\mathcal{U}_z(\cdot)$ for $\mathcal{U}(\cdot)$ by using:
\begin{align}
    % \cos x &= \frac{\exp^{ix}}{2} + \frac{\exp^{-ix}}{2} \\
    % \sin x &= i \frac{\exp^{-ix}}{2} - i \frac{\exp^{ix}}{2}
    \cos x &= \frac{\exp^{ix} + \exp^{-ix}}{2} \\
    \sin x &= \frac{\exp^{-ix} - \exp^{ix}}{2\ch{i}}
\end{align}
Then, we have:
\begin{equation}
    \mathcal{U}_z(\mathbf{a}_i) : \mathbf{a}_i \mapsto  
    \frac{1}{2}\begin{bmatrix} 
    \substack{
        \big( a_{1} e(+,1,i) + a_{1} e(-,1,i) \\ - a_{2} i e(-,1,i) + a_{2} i e(+,1,i) \big)
    } \\ 
    \substack{
        \big( a_{2} e(+,1,i) + a_{2} e(-,1,i) \\ + a_{1} i e(-,1,i) - a_{1} i e(+,1,i) \big)
    } \\ 
    \vdots \\ 
    \substack{
        \big( a_{D-1} e(+,D/2,i) + a_{D-1} e(-,D/2,i) \\ - a_{D} i e(-,D/2,i) + a_{D} i e(+,D/2,i) \big)
    } \\ 
    \substack{
        \big( a_{D} e(+,D/2,i) + a_{D} e(-,D/2,i) \\ + a_{D-1} i e(-,D/2,i) - a_{D-1} i e(+,D/2,i) \big)
    } \\ 
    \end{bmatrix}^\top
\end{equation}
where we used the function $e(+,j,k) = \exp^{2 \pi i f_j p_k}$ and $e(-,j,k) = \exp^{-2 \pi i f_j p_k}$.

The complex-valued pooled feature transform $\mathcal{C}_z(\mathbf{a}_i)$ corresponding to $\mathcal{U}_z(\mathbf{a}_i)$ can be obtained by adding up all the dimensions in $\mathcal{U}_z(\mathbf{a}_i)$:
\begin{equation}
    \mathcal{C}_z(\mathbf{a}_i) : \mathbf{a}_i \mapsto
    \frac{1}{2}\begin{bmatrix} 
    \sum_{d=1}^{D/2}
    \substack{
    \big( a_{2d-1} (1-i) + a_{2d} (1+i) \big) \exp^{2 \pi i f_d p_i}\\+ \big( a_{2d-1} (1+i) + a_{2d} (1-i) \big) \exp^{-2 \pi i f_d p_i}
    }
    \end{bmatrix}^\top
\end{equation}
Then, $\mathcal{C}_z(\mathbf{q}_m) \mathcal{C}_z(\mathbf{k}_n)^\top$ can be calculated as:
\begin{align*}
    \mathcal{C}_z(\mathbf{q}_m) &\mathcal{C}_z(\mathbf{k}_n)^\top = \\ & \Bigg[ \frac{1}{2} \sum_{d=1}^{D/2} \Big\{ \big( q_{2d-1} (1-i) + q_{2d} (1+i) \big) \exp^{2 \pi i f_d p_m} + \\ &\big( q_{2d-1} (1+i) + q_{2d} (1-i) \big) \exp^{-2 \pi i f_d p_m} \Big\} \Bigg] \cdot \\ &\Bigg[\frac{1}{2}\sum_{d=1}^{D/2}\Big\{ \big( k_{2d-1} (1-i) + k_{2d} (1+i) \big) \exp^{2 \pi i f_d p_n} + \\ &\big( k_{2d-1} (1+i) + k_{2d} (1-i) \big) \exp^{-2 \pi i f_d p_n} \Big\}\Bigg]
\end{align*}
Resolving this product will lead to a sum of four terms. We can again use the orthogonality of complex exponentials to obtain:
\begin{align*}
    \mathcal{C}_z&(\mathbf{q}_m) \mathcal{C}_z(\mathbf{k}_n)^\top = \frac{1}{4} \sum_{d=1}^{D/2} \\
    &\big( q_{2d-1} (1-i) + q_{2d} (1+i) \big) \\&\big( k_{2d-1} (1-i) + k_{2d} (1+i) \big) \exp^{2 \pi i f_d (p_m+p_n)} + \\
    &\big( q_{2d-1} (1-i) + q_{2d} (1+i) \big) \\&\big( k_{2d-1} (1+i) + k_{2d} (1-i) \big) \exp^{2 \pi i f_d (p_m-p_n)} + \\
    &\big( q_{2d-1} (1+i) + q_{2d} (1-i) \big) \\&\big( k_{2d-1} (1-i) + k_{2d} (1+i) \big) \exp^{-2 \pi i f_d (p_m-p_n)} + \\
    &\big( q_{2d-1} (1+i) + q_{2d} (1-i) \big) \\&\big( k_{2d-1} (1+i) + k_{2d} (1-i) \big) \exp^{-2 \pi i f_d (p_m+p_n)}
\end{align*}
We can use the following to simplify each of the four terms:
\begin{align*}
    (1 + i)^2 &= 2i \\
    (1 - i)^2 &= -2i \\
    (1 + i)(1-i) &= 2 \\
\end{align*}
and we obtain:
\begin{align*}
    \mathcal{C}_z(\mathbf{q}_m) \mathcal{C}_z&(\mathbf{k}_n)^\top = \frac{1}{2} \sum_{d=1}^{D/2} \\
    &\big( - i q_{2d-1} k_{2d-1} + q_{2d-1} k_{2d} +  q_{2d} k_{2d-1} + i q_{2d} k_{2d} \big)\\&\exp^{2 \pi i f_d (p_m+p_n)} + \\
    &\big( q_{2d-1} k_{2d-1} - i q_{2d-1} k_{2d} + i q_{2d} k_{2d-1} + q_{2d} k_{2d} \big)\\&\exp^{2 \pi i f_d (p_m-p_n)} + \\
    &\big( q_{2d-1} k_{2d-1} + i q_{2d-1} k_{2d} - i q_{2d} k_{2d-1} + q_{2d} k_{2d} \big)\\&\exp^{-2 \pi i f_d (p_m-p_n)} + \\
    &\big( i q_{2d-1} k_{2d-1} + q_{2d-1} k_{2d} + q_{2d} k_{2d-1} - i q_{2d} k_{2d} \big)\\&\exp^{-2 \pi i f_d (p_m+p_n)} \numberthis \label{eq:rope_pooled_attn_imaginary}
\end{align*}
The real-valued counterpart of this is $\mathfrak{Re} \big( \mathcal{C}_z(\mathbf{q}_m) \mathcal{C}_z(\mathbf{k}_n)^\top \big) = \mathcal{C}(\mathbf{q}_m) \mathcal{C}(\mathbf{k}_n)^\top$, which is:
\begin{align*}
    \mathcal{C}(\mathbf{q}_m) \mathcal{C}&(\mathbf{k}_n)^\top = \sum_{d=1}^{D/2} \Big\{ \\ 
    &(q_{m,2d-1} k_{n,2d-1} + q_{m,2d} k_{n,2d}) \cos \big( 2 \pi f_d (p_m - p_n) \big) + \\
    &(q_{m,2d-1} k_{n,2d} - q_{m,2d} k_{n,2d-1}) \sin \big( 2 \pi f_d (p_m - p_n) \big) + \\
    &(q_{m,2d-1} k_{n,2d-1} - q_{m,2d} k_{n,2d}) \sin \big( 2 \pi f_d (p_m + p_n) \big) + \\
    &(q_{m,2d-1} k_{n,2d} + q_{m,2d} k_{n,2d-1}) \cos \big( 2 \pi f_d (p_m + p_n) \big) \Big\}
\end{align*}

Note that, we do not prove this here, but we can show that $\mathcal{U}(\mathbf{q}_m) \mathcal{U}(\mathbf{k}_n)^\top \neq \mathcal{C}(\mathbf{q}_m) \mathcal{C}(\mathbf{k}_n)^\top$, which is precisely the fact that RoPE lacks the cross-dimension independent property (also illustrated in Fig. \ref{fig:drawing}). \qed \\

\noindent\textbf{IV. Derivations for toy example} corresponding to Equations (24), (25) and (26).\\

\noindent For RoPE, we can derive the expression as:
\begin{align*}
    a_{mn} \approx & \sum_{d=1}^{D/2} (q_{m,2d-1} k_{n,2d-1} + q_{m,2d} k_{n,2d} )
    \cos \Delta^-_d  + \\ &
    ( q_{m,2d-1} k_{n,2d} - q_{m,2d} k_{n,2d-1} )
    \sin \Delta^-_d\\
    = & 
    \sum_{d=1}^{D/2} \left[ \begin{array}{cc}
     q_{m, 2d-1} & q_{m, 2d}
    \end{array}\right]
    \left[ \begin{array}{c}
     k_{n, 2d-1} \\ k_{n, 2d}
    \end{array}\right]\cos \Delta^-_d + \\ & \left[ \begin{array}{cc}
     q_{m, 2d-1} & q_{m, 2d}
    \end{array}\right]
    \left[ \begin{array}{c}
     k_{n, 2d} \\ - k_{n, 2d-1}
    \end{array}\right]\sin \Delta^-_d\\
    = &
    \sum_{d=1}^{D/2} \left[ \begin{array}{cc}
    \cos \psi_q^d & \sin \psi_q^d
    \end{array}\right]
    \left[ \begin{array}{c}
     \cos \psi_k^d \\ \sin \psi_k^d
    \end{array}\right]\cos \Delta^-_d \\ & + 
    \left[ \begin{array}{cc}
     \cos \psi_q^d & \sin \psi_q^d
    \end{array}\right]
    \left[ \begin{array}{c}
     \sin \psi_k^d \\ - \cos \psi_k^d
    \end{array}\right]\sin \Delta^-_d\\
    = &
    \sum_{d=1}^{D/2} \cos (\psi_q^d - \psi_k^d )\cos \Delta^-_d + \sin (\psi_k^d - \psi_q^d ) \sin \Delta^-_d\\
    = &
    \sum_{d=1}^{D/2} \cos (\psi_q^d - \psi_k^d )\cos \Delta^-_d - \sin (\psi_q^d - \psi_k^d ) \sin \Delta^-_d\\
    = & \sum_{d=1}^{D/2} \cos \big( ( \psi_q^d - \psi_k^d ) + f_d ( \xi_m^d - \xi_n^d ) \big)
\end{align*} 
where $\Delta^-_d = f_d ( \mathcal{P}_Q[m] - \mathcal{P}_K[n] ) = f_d ( \xi_m^d - \xi_n^d )$.

For F-StrIPE$_1$, we can derive the expression as:
\begin{align*}
    a_{mn} \approx & \sum_{d=1}^D q_{md} k_{nd} \cos \Delta^-_d \\
    = & 
    \sum_{d=1}^{2/D} \left[ \begin{array}{cc}
     q_{m, 2d-1} & q_{m, 2d}
    \end{array}\right] \left[ \begin{array}{c}
     k_{n, 2d-1} \\ k_{n, 2d}
    \end{array}\right] \cos \Delta^-_d\\
    = & 
    \sum_{d=1}^{2/D} \left[ \begin{array}{cc}
     \cos \psi_q^d & \sin \psi_q^d
    \end{array}\right] \left[ \begin{array}{c}
     \cos \psi_k^d \\ \sin \psi_k^d
    \end{array}\right] \cos \Delta^-_d\\
    = & 
    \sum_{d=1}^{2/D} 
     \cos (\psi_q^d - \psi_k^d) \cos (f_d(\xi_m^d - \xi_n^d))\\
\end{align*}
where $\Delta^-_d = f_d ( \xi_m^d - \xi_n^d )$.

For RoPEPool, we can derive the expression as:
 \begin{align*}
    a_{mn} \approx & \sum_{d=1}^{D/2} \Big\{(q_{m,2d-1} k_{n,2d-1} + q_{m,2d} k_{n,2d}) \cos \Delta^-_d \hspace{1mm} + \\ & (q_{m,2d-1} k_{n,2d} - q_{m,2d} k_{n,2d-1}) \sin \Delta^-_d \hspace{1mm} + \\
    &(q_{m,2d-1} k_{n,2d-1} - q_{m,2d} k_{n,2d}) \sin \Delta^+_d \hspace{1mm} + \\ & 
    (q_{m,2d-1} k_{n,2d} + q_{m,2d} k_{n,2d-1}) \cos \Delta^+_d \Big\}\\
    %%%%%%%%%%%%%%%%%%%%%%%%%%
    = &
    \sum_{d=1}^{D/2} \Big\{ \left[ \begin{array}{cc}
     q_{m, 2d-1} & q_{m, 2d}
    \end{array}\right]
    \left[ \begin{array}{c}
     k_{n, 2d-1} \\ k_{n, 2d}
    \end{array}\right]\cos \Delta^-_d + \\ & 
    \left[ \begin{array}{cc}
     q_{m, 2d-1} & q_{m, 2d}
    \end{array}\right]
    \left[ \begin{array}{c}
     k_{n, 2d} \\ -k_{n, 2d-1}
    \end{array}\right]\sin \Delta^-_d + \\
     & 
    \left[ \begin{array}{cc}
     q_{m, 2d-1} & q_{m, 2d}
    \end{array}\right]
    \left[ \begin{array}{c}
     k_{n, 2d-1} \\ - k_{n, 2d}
    \end{array}\right]\sin \Delta^+_d + \\ & \left[ \begin{array}{cc}
     q_{m, 2d-1} & q_{m, 2d}
    \end{array}\right]
    \left[ \begin{array}{c}
     k_{n, 2d} \\ k_{n, 2d-1}
    \end{array}\right]\cos \Delta^+_d \Big\}\\
    %%%%%%%%%%%%%%%%%%%%%%%%%%
    = & 
    \sum_{d=1}^{D/2} \left[ \begin{array}{cc}
    \cos \psi_q^d & \sin \psi_q^d
    \end{array}\right]
    \left[ \begin{array}{c}
     \cos \psi_k^d \\ \sin \psi_k^d
    \end{array}\right]\cos \Delta^-_d 
    + \\ & 
    \left[ \begin{array}{cc}
     \cos \psi_q^d & \sin \psi_q^d
    \end{array}\right]
    \left[ \begin{array}{c}
     \sin \psi_k^d \\ -\cos \psi_k^d \\
    \end{array}\right]\sin \Delta^-_d + \\
     & 
    \left[ \begin{array}{cc}
    \cos \psi_q^d & \sin \psi_q^d
    \end{array}\right]
    \left[ \begin{array}{c}
     \cos \psi_k^d \\ - \sin \psi_k^d
    \end{array}\right]\sin \Delta^+_d + \\ & 
    \left[ \begin{array}{cc}
    \cos \psi_q^d & \sin \psi_q^d 
    \end{array}\right]
    \left[ \begin{array}{c}
     \sin \psi_k^d \\ \cos \psi_k^d
    \end{array}\right]\cos \Delta^+_d\\
    %%%%%%%%%%%%%%%%%%%%%%%%%%
    = &
    \sum_{d=1}^{D/2} \cos (\psi_q^d - \psi_k^d )\cos \Delta^-_d \\ & 
    - 
    \sin (\psi_q^d - \psi_k^d ) \sin \Delta^-_d \\ & 
    + 
    \cos (\psi_q^d + \psi_k^d )\sin \Delta^+_d \\ & 
    + \sin (\psi_q^d + \psi_k^d ) \cos \Delta^+_d\\
    %%%%%%%%%%%%%%%%%%%%%%%%%%
    = & 
     \sum_{d=1}^{D/2} \cos (\psi_q^d - \psi_k^d + \Delta^-_d ) + \sin (\psi_q^d + \psi_k^d + \Delta^+_d )\\ 
    = & \sum_{d=1}^{D/2} \cos (\psi_q^d - \psi_k^d + f_d(\xi_m^d - \xi_n^d)) \\ & + \sin (\psi_q^d + \psi_k^d + f_d(\xi_m^d + \xi_n^d) )\\
    = & \sum_{d=1}^{D/2} \cos ((\psi_q^d + f_d\xi_m^d) - (\psi_k^d + f_d\xi_n^d)) \\ & + \sin ((\psi_q^d + f_d\xi_m^d) + (\psi_k^d + f_d\xi_n^d))\\
    = & \sum_{d=1}^{D/2} \cos ((\psi_q^d + f_d\xi_m^d) - (\psi_k^d + f_d\xi_n^d)) +\\ &  \cos ((\psi_q^d + f_d\xi_m^d) + (\psi_k^d + f_d\xi_n^d) - \frac{\pi}{2})\\
    %%%%%%%%%%%%%%%%%%%%%%%%%%
    & [ \text{Use} \cos X + \cos Y = 2 \cos ( \frac{X+Y}{2} ) \cos ( \frac{X-Y}{2} ) ] \\
    % = & \sum_{d=1}^{D/2} 2 \cos \left( \frac{A - B}{2} + \frac{\pi}{4} \right) \cos \left( \frac{A + B}{2} + \frac{\pi}{4} \right)\\
    %%%%%%%%%%%%%%%%%%%%%%%%%%
    = & \sum_{d=1}^{D/2} 2 \cos \left( \psi_q^d + f_d \xi_m^d - \frac{\pi}{4} \right) \cos \left( \psi_k^d + f_d \xi_n^d - \frac{\pi}{4} \right)
\end{align*}
% where 
% \begin{align*}
% A &= \psi_q^d - \psi_k^d - f_d(\xi_m^d - \xi_n^d) \\
% B &= \psi_q^d + \psi_k^d + f_d(\xi_m^d + \xi_n^d)
% \end{align*}
